# Supplementary material for: Learning Task Decomposition with Ordered Memory Policy Network
Source: arXiv:2103.10972 source file (2021-03-19)
Supplement: Supplementary file 1 [file setup.tex]

\section{Experiment Setup}
We use a one-layer GRU to encode the sketch and concatenate it with the observation.
